# Supplementary material for: Anomalous charge transport of superconducting Cu$_{x}$PdTe$_2$ under high pressure
Source: arXiv:2106.05613 source file (2021-06-10)
Supplement: Supplementary file 1 [file supplemental_material.pdf]

# Supplemental material

# Anomalous charge transport of superconducting $Cu_xPdTe_2$ under high pressure

Hancheng Yang,[1] M. K. Hooda,[2] C. S. Yadav,[2] David Hrabovsky,[3] Andrea Gauzzi,[1] and Yannick Klein[1,*]

*[1]IMPMC, Sorbonne Université and CNRS, 4 place Jussieu, 75005 Paris, France*

*[2]School of Basic Sciences, Indian Institute of Technology Mandi, Mandi-175005 (H.P.), India*

*[3]Plateforme Mesures Physiques à Basses Températures (MPBT), Sorbonne Université, 4 place Jussieu 75005 Paris, France*

(Dated: April 25, 2021)

PACS numbers: 74.62.Fj,52.25.Fi,74.25.-q

## ANALYSIS OF THE LOW-TEMPERATURE RESISTIVITY DATA

In the present Supplemental Information section, we provide details of the above analysis leading to the conclusion on the unusual $T^4$ power law in $PdTe_2$ and $Cu_{0.05}PdTe_2$. In Fig. S1 we first plot the normalized raw resistivity data $\rho(T)/\rho(300K)$ as a function of $T^4$ at different pressures. The linear dependence of these curves is evident for both PdTe2 and Cu0.05PdTe2 and for all pressures at least in the 2-20 K range, i.e. over one decade, as indicated by the agreement of the experimental data with a simple linear fit using the function $\rho(T)/\rho(300K) = C + AT^4$.

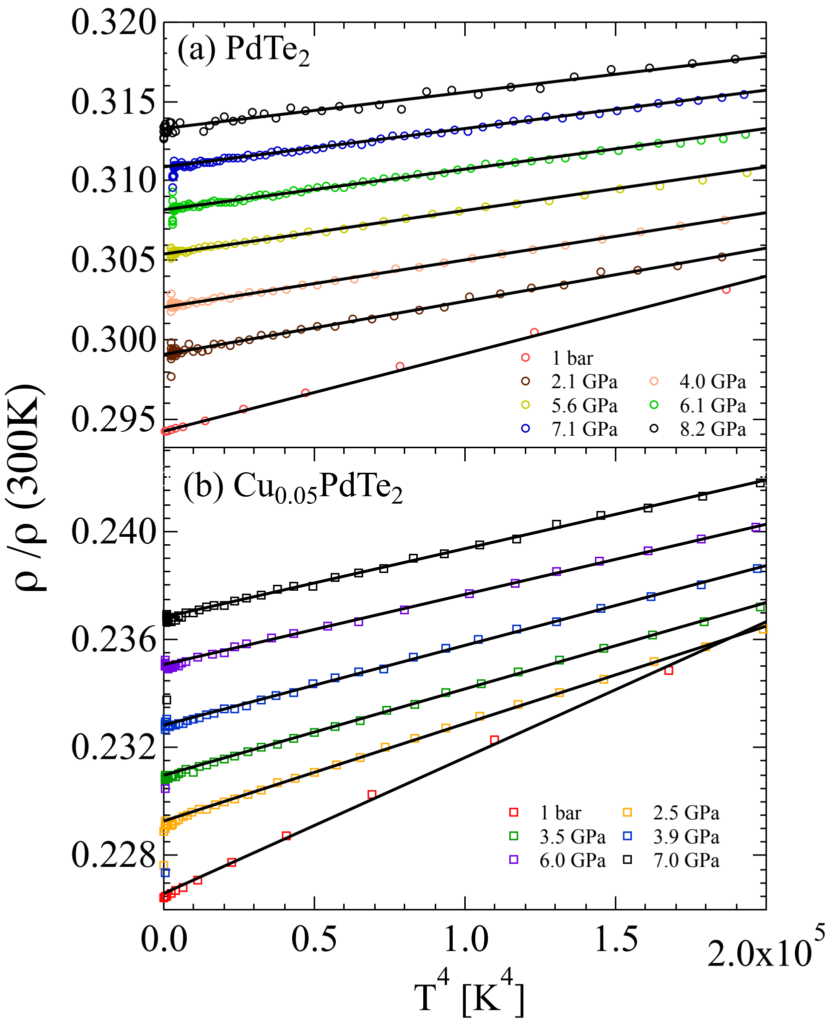


FIG. 1: Low-temperature normalized resistivity of $PdTe_2$ and $Cu_{0.05}PdTe_2$ as a function of $T^4$ measured at different pressures. Black lines are best linear fits. Data are shifted vertically for clarity.

As a further verification of the validity of the $T^4$ power law, we fit the same data using the

function $\rho(T)/\rho(300K) = C + AT^4$ where the exponent $n$ is now a free parameter. The experimental and fitting curves are plotted in Fig. S2. The numerical parameters of the fit are given in Tables S1 and S2. The result is very convincing again for both samples and at all pressures: the fit reproduces very well the data and yields $n = 4$ within the uncertainty of the fit.

The fit allows us to estimate the normalized residual resistivity value $C$ in a reliable manner and thus to subtract it from the normalized $\rho/\rho(300K)$ curves and to plot the resulting $\Delta\rho/\rho(300K)$ as a function of $T$ in a log-log scale, which we have done in Fig. 4 of the main article.

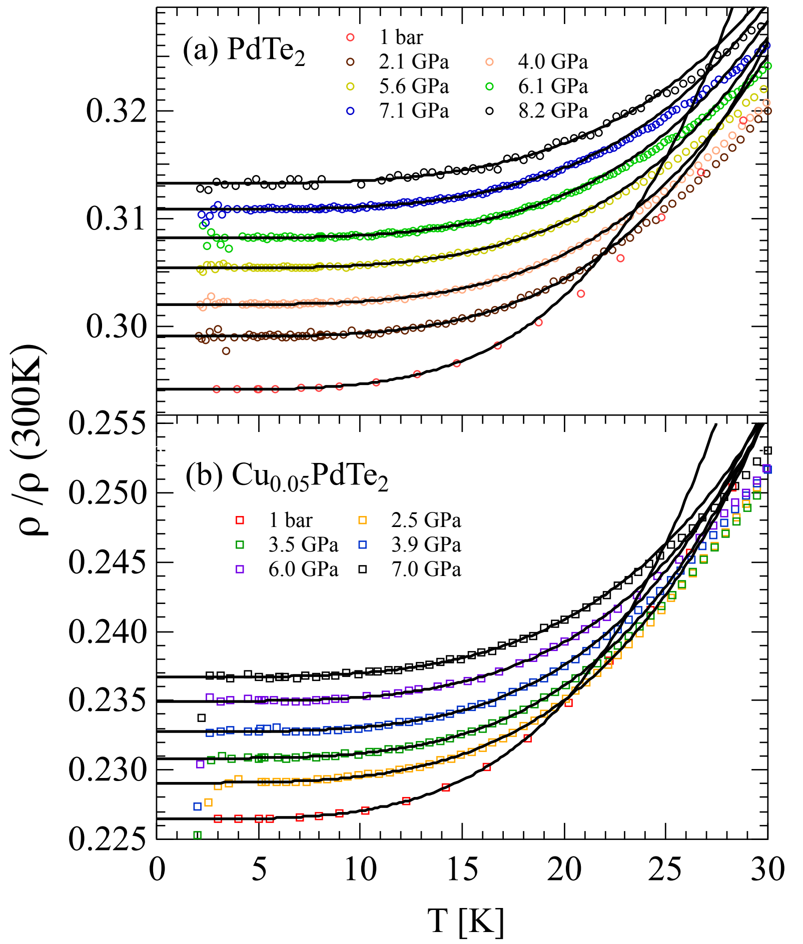


FIG. 2: Normalized resistivity of $PdTe_2$ and $Cu_{0.05}PdTe_2$ measured at different pressures as a function of temperature. Black curves are best fits using the function $\rho(T)/\rho(300K) = C + AT^n$, where $n$ is a free parameter. The results of the fit are given in Tables S1 and S2.

| Pressure [GPa] | $C$ | $A \times 10^{-8}$ | $n$ | Fitting range [K] |
|---|---|---|---|---|
| 0 | 0.079112(5) | 4.4(5) | 4.07(4) | 2 - 18 |
| 2.1(1) | 0.15703(3) | 2.9(6) | 4.04(8) | 4 - 20 |
| 4.0(2) | 0.19699(2) | 3.5(6) | 3.93(5) | 5 - 20 |
| 5.6(2) | 0.22538(1) | 2.9(6) | 3.97(7) | 5 - 20 |
| 6.1(3) | 0.24967(2) | 2.7(6) | 3.98(7) | 4 - 20 |
| 7.1(3) | 0.27081(2) | 2.8(6) | 3.95(7) | 3.5 - 20 |
| 8.2(5) | 0.31024(7) | 3(1) | 3.9(2) | 3 - 20 |

TABLE 1: Fitting parameters for $PdTe_2$. Numbers in parenthesis indicate statistical uncertainty.

| Pressure [GPa] | $C$ | $A \times 10^{-8}$ | $n$ | Fitting range [K] |
|---|---|---|---|---|
| 0 | 0.044454(6) | 8.8(7) | 3.83(3) | 2 - 20 |
| 2.5(1) | 0.12711(2) | 7(1) | 3.77(5) | 4 - 20 |
| 3.5(2) | 0.16583(1) | 4.9(7) | 3.87(5) | 2.6 - 20 |
| 3.9(2) | 0.19276(2) | 3.2(9) | 3.97(9) | 2.6 - 20 |
| 6.0(3) | 0.22396(2) | 3.8(9) | 3.88(8) | 3- 20 |
| 7.0(4) | 0.23669(2) | 5(1) | 3.79(8) | 2.6 - 20 |

TABLE 2: The same as above for $Cu_{0.05}PdTe_2$.

* yannick.klein@sorbonne-universite.fr
